# Supplementary material for: Pattern selection in reaction diffusion systems
Source: arXiv:2005.07940 source file (2020-09-15)
Supplement: Supplementary file 1 [file supplement.pdf]

**BACKGROUND INFORMATION**

We consider the following reaction-diffusion toy-model,

$$\frac{\partial u}{\partial t} = D_u \frac{\partial^2 u}{\partial x^2} - \beta u(u+v)^2 + \gamma v + \delta c - \delta u, \tag{1a}$$

$$\frac{\partial v}{\partial t} = D_v \frac{\partial^2 v}{\partial x^2} + \beta u(u+v)^2 - \gamma v - \delta v, \tag{1b}$$

with real parameters $D_u > D_v > 0$, $\beta, \gamma, c > 0$ and $\delta \geq 0$ and reflexive boundary conditions at $x = \pm\frac{L}{2}$. It is easy to see from the above equations that the total mass at steady state is the same for any set of initial conditions i.e.,

$$\int_{-\frac{L}{2}}^{\frac{L}{2}} \bar{u} + \bar{v}\; dx = c,$$

where $\bar{u}$ and $\bar{v}$ are the steady state concentrations. We implement the following non-dimensionalisation:

$$u \to \frac{u}{c}, \quad v \to \frac{v}{c}, \quad x \to \frac{x}{L}, \quad t \to \frac{D_v}{L^2} t,$$

to obtain

$$\frac{\partial u}{\partial t} = d\frac{\partial^2 u}{\partial x^2} + \Gamma\left(-au(u+v)^2 + v + b(1-u)\right) \tag{2a}$$

$$\frac{\partial v}{\partial t} = \frac{\partial^2 v}{\partial x^2} + \Gamma\left(au(u+v)^2 - (1+b)v\right)\ , \tag{2b}$$

in terms of the dimensionless variables,

$$a = \frac{\beta c^2}{\gamma}, \quad b = \frac{\delta}{\gamma}, \quad \Gamma = \frac{\gamma L^2}{D_v}, \quad d = \frac{D_u}{D_v}. \tag{3}$$

Let us perform linear stability analysis on the system. In the absence of diffusion there is a single fixed point

$$u_0 = \frac{b+1}{a+b+1}, \quad v_0 = \frac{a}{a+b+1}.$$

The Jacobian at this point is given by

$$\begin{aligned} J =& \Gamma \begin{bmatrix} f_u & f_v \\ g_u & g_v \end{bmatrix}_{(u_0, v_0)} \\ =& \Gamma \begin{bmatrix} -a - 2au_0 - b & 1 - 2au_0 \\ a + 2au_0 & 2au_0 - 1 - b \end{bmatrix}. \end{aligned} \tag{4}$$

where $f$ and $g$ are the reaction terms in Eq. (2a) and Eq. (2b) respectively. The trace and determinant of the Jacobian are easily found to be

$$TrJ = \Gamma(-a-1-2b)$$
$$DetJ = \Gamma^2(b\,(a+b+1)).$$

Since, $TrJ < 0$ and $DetJ > 0$, the homogeneous fixed point is always stable in the absence of diffusion for any set of parameters $a, b, \Gamma > 0$. For the mass-conserved case $b = 0$, the determinant vanishes. This is due to a zero eigenvalue, the eigenvector of which does not obey the conservation condition. The other eigenvector corresponds to the mass-conserving direction $(1, -1)^T$ and has eigenvalue $f_u - f_v = -a < 0$. Hence, the base state is stable with respect to perturbations preserving mass conservation.

Following the standard approach [1], we now consider a spatial perturbation around the uniform state $u = u_0 + \delta u$, $v = v_0 + \delta v$ in presence of diffusion. The evolution of this can perturbation $\boldsymbol{w} = \begin{pmatrix} \delta u \\ \delta v \end{pmatrix}$ can be written as

$$\boldsymbol{w}(x,t) = \sum_k \boldsymbol{c}_k \exp^{\sigma_k t} \epsilon_k(x)\ ,$$

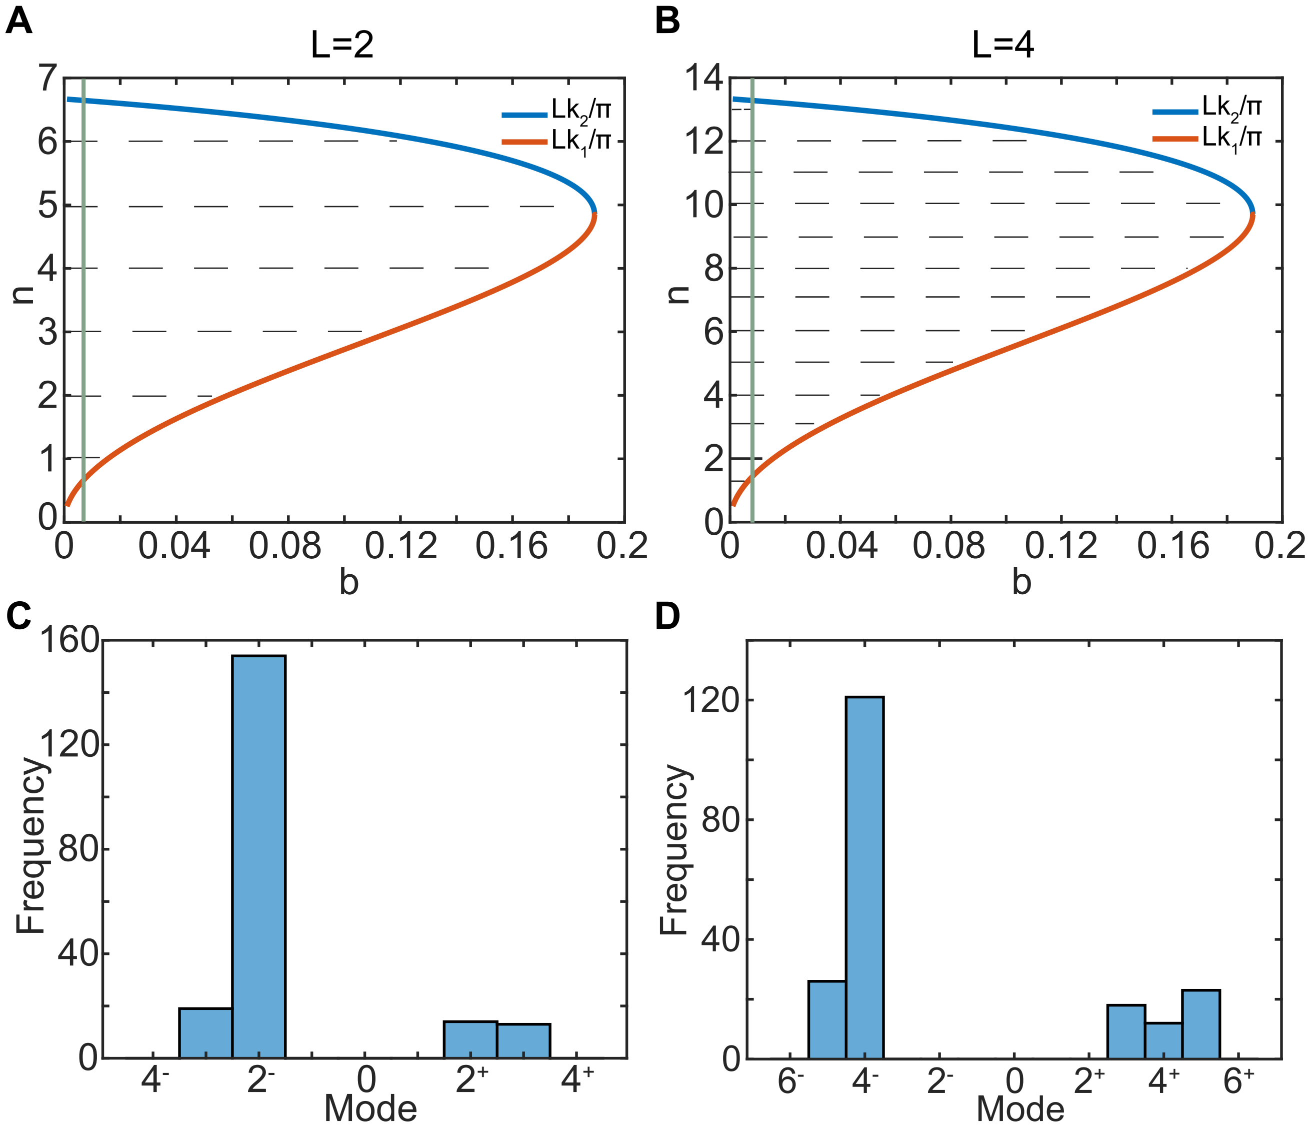


FIG. S1. **Instability regions and dominant phase of the pattern.**
($A$,$B$). We find that a broad range of modes are unstable for different parameters. Plotted is the region of instability (see also Fig 1D in main text) as a function of $b$ with $a = 3.75$. $k_1$ and $k_2$ are the bounds of instability as defined by Eq. (9). The horizontal dashed lines indicate the discrete modes that fit in the range. The vertical green line represents our default value of $b = 0.0039$. $L = 2$ and $L = 4$ in ($A$) and ($B$) respectively. ($C$,$D$). The system was solved for 200 different initial random perturbations of the uniform base state with $L = 2$ ($C$) and $L = 4$ ($D$). The phase of the pattern (the sign of the amplitude of the dominant mode) is indicated by a minus or plus sign. The steady state pattern is dominated by a mode lower ($n = 2$ and $n = 4$) than what is predicted by the linear stability analysis ($n = 4$ and $n = 8$ respectively). The growth rate of each mode for $L = 4$ is shown in Fig. 1D. In ($C$) and ($D$) we use our default parameter set stated in the Methods section.

where the $\epsilon_k$ are the eigenfunctions of the Laplacian

$$\nabla^2 \epsilon_k(x) = -k^2 \epsilon_k(x) \tag{5}$$

subject to the given boundary conditions. Inserting this into the equation Eq. (2) and linearizing around the homogeneous steady state we obtain the eigenvalue problem

$$\left| J - k^2 D - \sigma_k \mathbf{I} \right| = 0 \quad \text{where } D = \begin{pmatrix} D_u & 0 \\ 0 & D_v \end{pmatrix} . \tag{6}$$

The conditions for the growth rate $\sigma_k$ to be positive for some range of wave numbers $k_1^2 < k^2 < k_2^2$ is given by [1]

$$f_u + dg_v > 2\sqrt{d(f_u g_v - f_v g_u)} \tag{7}$$

which we evaluate to find

$$d\frac{b+1}{a+b+1}(a-b-1) - \frac{a^2+b^2+4ab+3a+b}{a+b+1} - 2\sqrt{db(a+b+1)} > 0. \tag{8}$$

By a straightforward calculation, we also find

$$\begin{aligned} k_1^2 &= \frac{\Gamma}{2d}\left[(-a-2au_0-b+d(2a-1-b)) - \{(-a-2au_0-b+d(2a-1-b))^2 - 4db(a+b+1)\}^{1/2}\right] \\ k_2^2 &= \frac{\Gamma}{2d}\left[(-a-2au_0-b+d(2a-1-b)) + \{(-a-2au_0-b+d(2a-1-b))^2 - 4db(a+b+1)\}^{1/2}\right]. \end{aligned} \tag{9}$$

The inequality Eq. (8) relating $a$, $b$ and $d$ determines the parameter values for which there exists a band of unstable wave numbers i.e. the *Turing space*. However, for a finite domain the eigenvalues of the Laplacian are discrete. In particular, for the domain $[0, L]$ with reflexive boundary conditions, the wave number $k = \frac{n\pi}{L}$ for integer $n$ and the eigenfunctions are, labelling now by $n$, $\epsilon_n = \cos(\frac{n\pi x}{L})$. Since $k$ is discrete the condition Eq. (8) is a necessary but not sufficient for instability. A discrete mode $n$ with corresponding wave number $k = \frac{n\pi}{L}$ must exist within the range of instability $[k_1, k_2]$. Note that while $\Gamma$ does not enter into the condition Eq. (8), which, if any, discrete modes fall into the range $[k_1, k_2]$ does depend on $\Gamma$. In Fig. 1D, we show that region defined by Eq. (8) as well as the parameter regions in which each mode is unstable. We also show the instability region as function of $b$ in Fig. S1 for domain lengths of $L = 2$ and $L = 4$ (as used in Figs. 1 and 2).

## MOVEMENT OF POINT SINKS

We study the movement of points sinks numerically by initialising the sinks at arbitrary positions and solving Eq. (A15) and Eq. (B7) of the main text (See Figure S2, Figure 3B, Figure 3D). As above, we consider the regime in which the timescale of gradient formation is much faster than that of sink movement. The profile $A(x)$ can therefore be approximated by Eq. (A1).

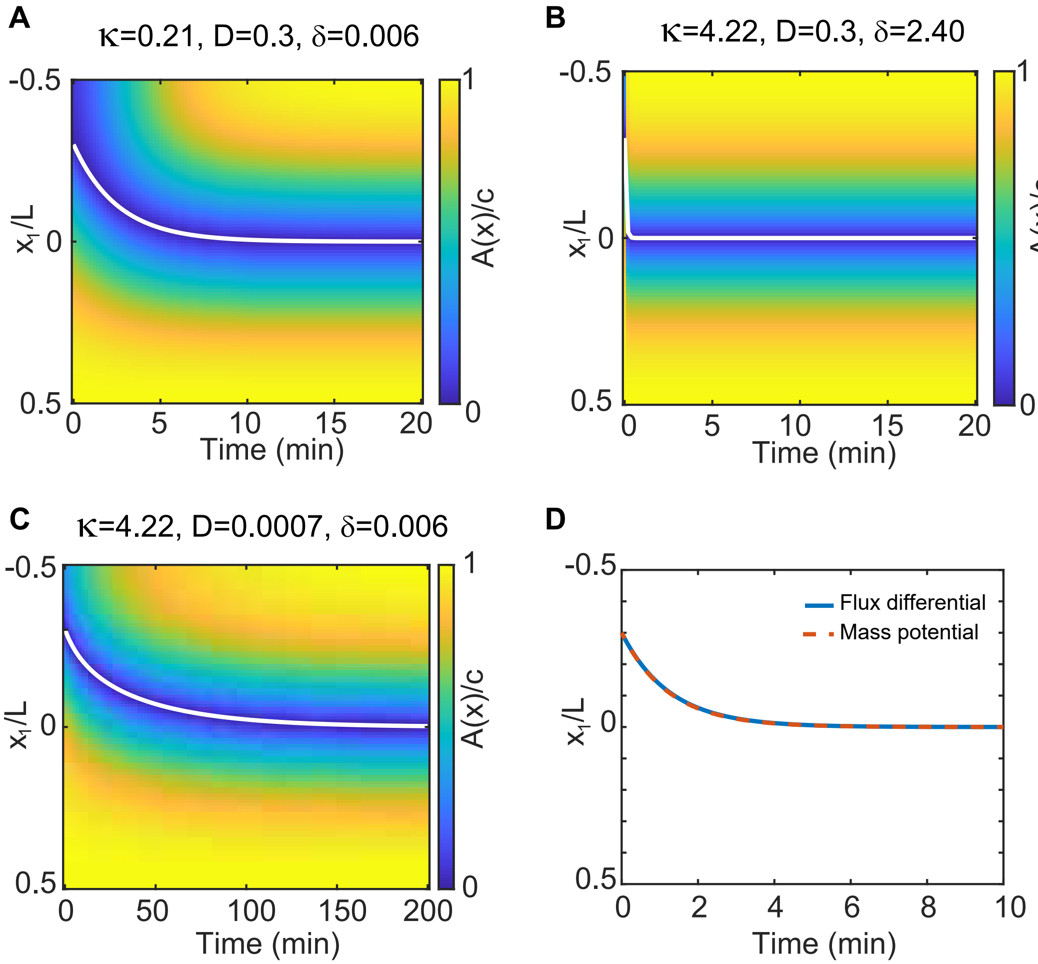


FIG. S2. **Point sink movement under changes in $\delta$ and $D$.**
($A$). Figure 3B reproduced for comparison. ($B$). With all other parameters remaining the same as in (A) $\kappa$ is increased by changing $\delta$. Sink moves faster to middle of the domain. This is because the flux through the system is increased. ($C$) Same as ($B$) but $\kappa$ is changed via $D$ instead of delta. In this case the higher value of $\kappa$ leads to slower movement. This is because the lower diffusive length-scale means that there is less flux exiting the system through the sink (and the total flux through the system ($c\delta L$) is unchanged). ($D$). A sample trajectory of sink (with parameters of $A$) is plotted in blue using Eq. (10) in the main text (dynamics due to flux differential). Overlaid dashed lines are the result of dynamics using Eq. (11) in main text, with the sink moving on a mass potential. Parameters: $\mu = 1, c = 1, \nu = 1$ across all panels. $\kappa$ and corresponding changes in $\delta$ and $D$ are indicated on top of each panel.

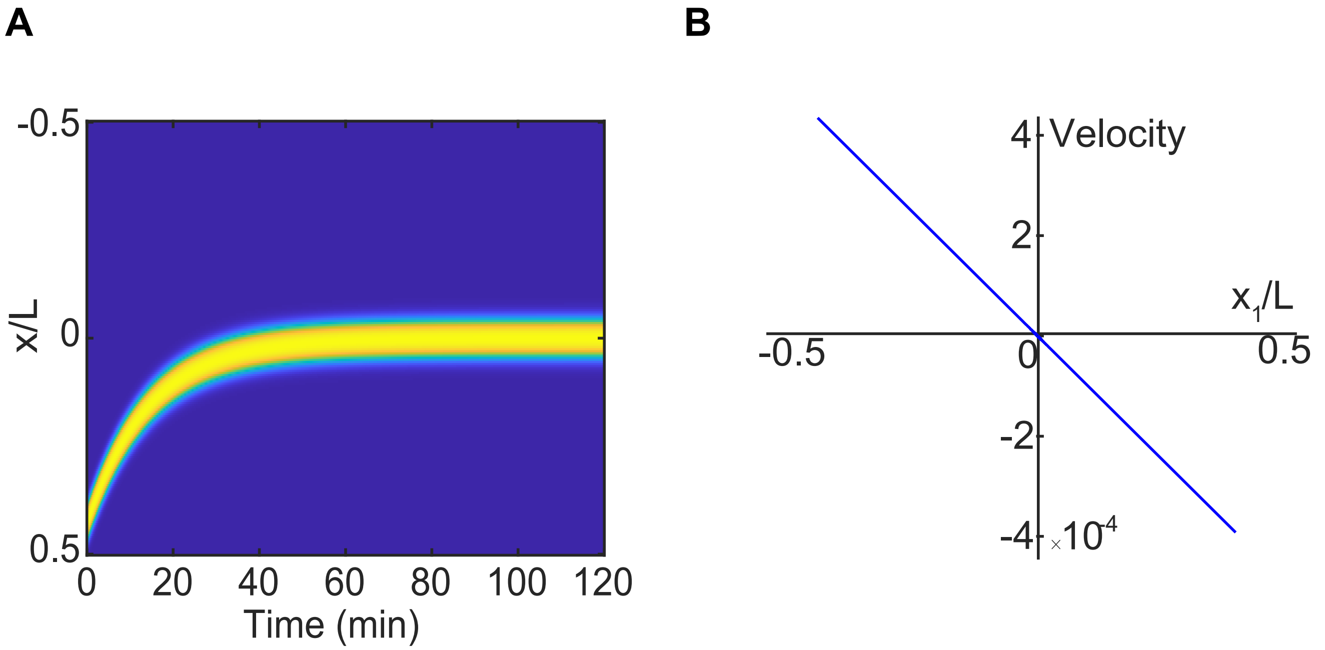


FIG. S3. **Movement of spikes in a Turing pattern**.
In the limit $D_v \to 0$ peaks become narrow spikes. ($A$). A single spike moves exponentially to the middle of the domain. ($B$). The spike velocity varies linearly with spike position over most of the domain. Parameters: Default, with $D_v = 0.0012$.

### Mass minimisation in the Turing system

In this section, we derive the prediction for the number of peaks in the steady state of the Turing system. In the singular (spike) limit Eq. (1), we obtain the following equation for the fast species $u$ at steady-state (Eq. (13) in main text)

$$D_u \frac{d^2u}{dx^2} + c\delta - \delta u - \sum_{i=1}^{n} \frac{\rho}{u} L\delta(x - x_i) = 0 \tag{10}$$

where $\rho = 6\frac{\sqrt{D_v}}{L}\frac{\delta\sqrt{\gamma+\delta}}{\beta}$. Note the inverse dependence on the variable in the sink term. Following the same approach as in the previous section, the solution of this equation is given by

$$u(x) = c - \sum_i \rho_i' G(x; x_i) \ , \tag{11}$$

with the Green's function as previously defined (with the equivalent dimensionless parameter $\kappa = L\sqrt{\frac{\delta}{D_u}}$) and where the $\rho_i'$ are determined by the $n$ algebraic equations

$$\rho_i' = \sigma \frac{c^2}{u(x_i)} \ , \tag{12}$$

where $\sigma = \frac{\rho}{c^2\delta}$ is a dimensionless parameter. Let us consider the case where the sinks are regularly positioned and of the same strength i.e. $\boldsymbol{x} = \bar{\boldsymbol{x}}$ and $\rho_i' = \rho'$. This implies,

$$u(x_i) = c - \sum_j \rho_j' G(x_i; x_j) = c - \rho' \sum_j G(x_i; x_j).$$

We showed in the main text that

$$\sum_j G(x_i;x_j) = \frac{\kappa}{2}\coth(\frac{\kappa}{2n}).$$

As in the case of the point sinks the flux differential across the spikes vanishes for the regularly positioned configuration $\Delta J_i(\bar{\boldsymbol{x}}) = 0$. We then have

$$\rho' = \frac{\sigma c^2}{(c - \rho' \frac{\kappa}{2}\coth\frac{\kappa}{2n})}. \tag{13}$$

Solving for $\rho'$, we find two solutions

$$\rho'_{\pm} = \frac{c}{\kappa\coth\left(\frac{\kappa}{2n}\right)}\left[1 \pm \sqrt{1 - 2\sigma\kappa\coth\left(\frac{\kappa}{2n}\right)}\right] \tag{14}$$

with corresponding total masses

$$M_{\pm} = \frac{1}{L}\int_{-\frac{L}{2}}^{\frac{L}{2}} u dx = c - n\rho'_{\pm}. \tag{15}$$

For a fixed set of parameters, we can thus calculate the predicted total mass of $u$ for a solution consisting of $n$ regularly positioned spikes. As we show in Fig. 5 (see also Fig. S4), this is minimised for a particular number of spikes. We also show that value of $n$ is an excellent predictor for the steady-state number of peaks obtained numerically (after any coarsening, see Fig. 5E) even when the peaks are not very spike-like (see Fig. S5F).

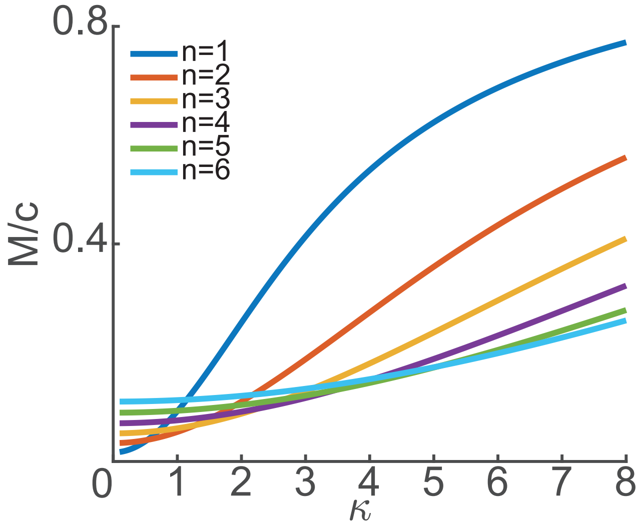


FIG. S4. Normalised total mass plotted as a function of $\kappa$ for different number of spikes. As $\kappa \to 0$, $M$ is minimal for a single spike. Parameters: Same as Fig. 5C,D,E in the main text

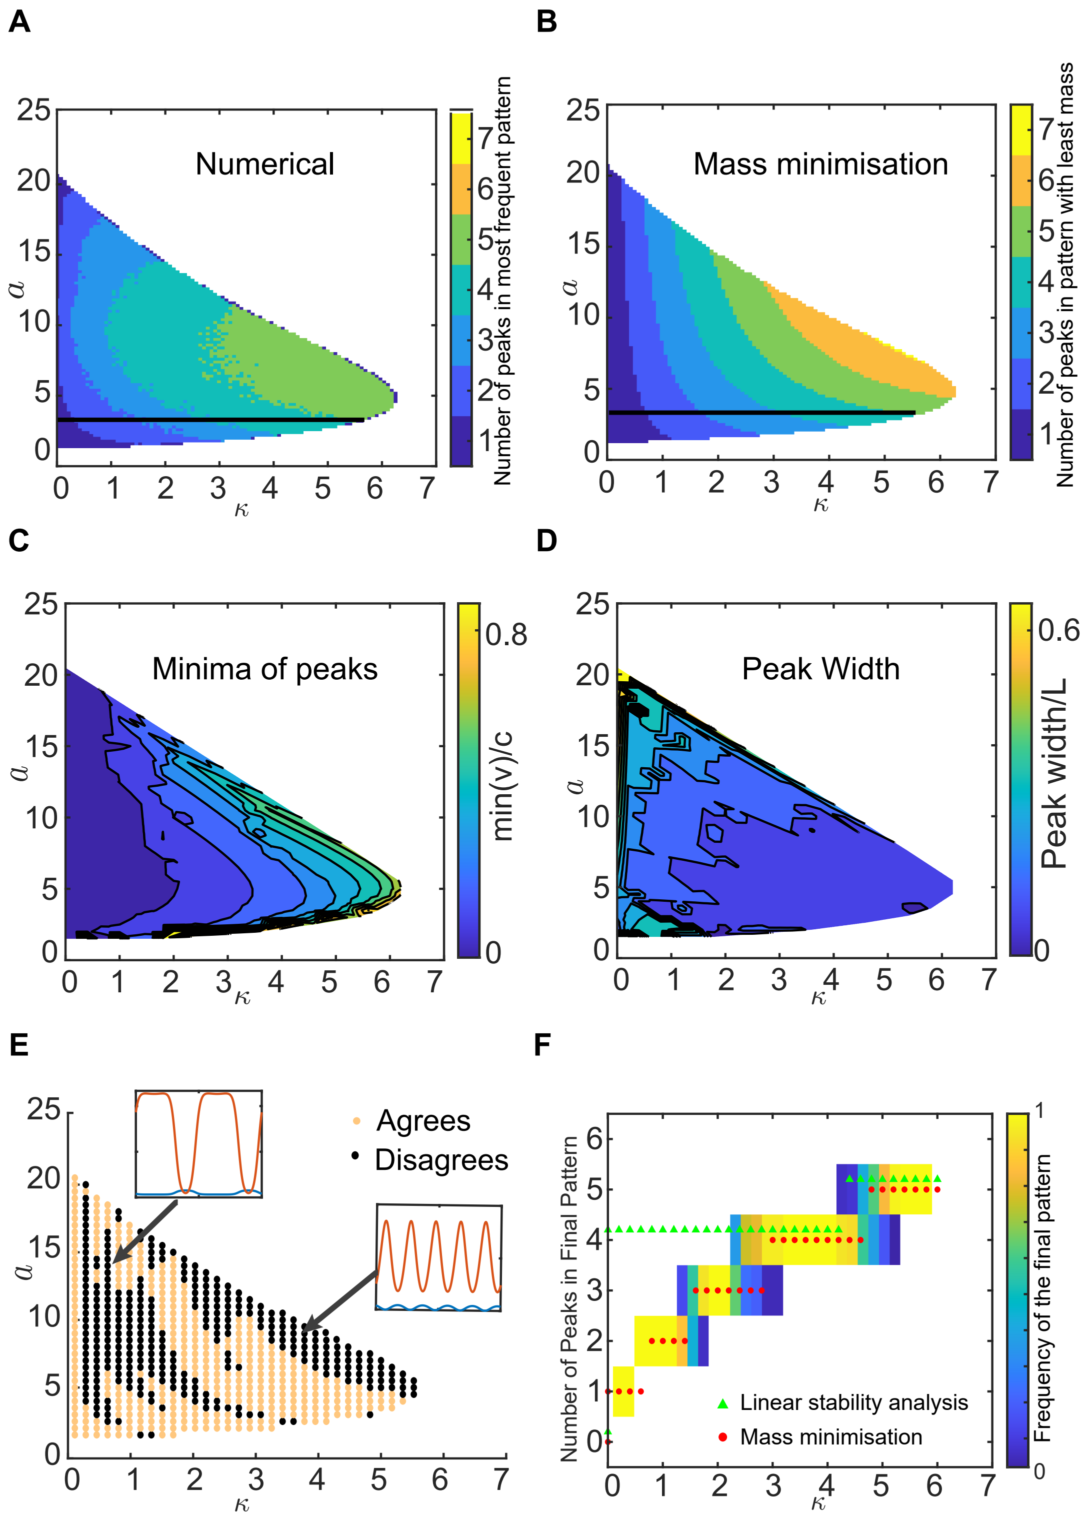


FIG. S5. **Comparing mass minimisation with numerical simulations**.
($A$). Fig. 5A is reproduced with a changed colorbar for comparison with the predictions from mass minimisation. ($B$). The number of peaks in the pattern with the lowest the total mass $M$ is plotted as a function of $a$ and $\kappa$. ($C$). Contours of minima of peaks ($min(v)/c$) of the steady state patterns from numerical simulations is plotted as a function of $a$ and $\kappa$. ($D$). Same as ($C$), with contours of *peak width* of the steady state patterns.($E$). We perform a direct comparison of results between numerical simulations in ($A$) and predictions in ($B$). The prediction is surprisingly accurate (beige dots) for large regions of the Turing space. Though, it is inaccurate (black dots) when $\kappa \gg 1$ or $a \gg 1$, as patterns have a baseline and peaks are now much broader respectively(see inset and ($C$,$D$)). ($F$). Same as Fig. 5E in the main text but for default parameters (peak like solutions). Mass minimisation correctly predicts the number of peaks at steady state, even though it is less accurate than the spike case in Fig. 5E. Data from 50 simulations with random perturbations from the homogeneous state for each parameter set. Parameters: Default with $L = 4$. For ($F$) we sweep across $\kappa$ (black line in ($A$) and ($B$)) for the default value of $a = 3.75$.

**Dynamics of a single spike**

In this section, we show the connection between the dynamics of peaks due to the flux differential and to mass potential for a single spike. Let us consider the general case (arbitrarily positioned) of a single spike. The solution is given by

$$u(x) = c - \rho_1' G(x; x_1). \tag{16}$$

where, for a given spike position $x_1$, there are two solutions for $\rho_1'$

$$\rho_{1\pm}' = \frac{c}{2G(x_1; x_1)} \left(1 \pm \sqrt{1 - 4\sigma G(x_1; x_1)}\right) \tag{17}$$

with

$$G(x_1; x_1) = \frac{\kappa}{2} \left[ \frac{\cosh(\frac{2\kappa x_1}{L})}{\sinh(\kappa)} + \coth(\kappa) \right] \tag{18}$$

The flux differential across the spike is given by,

$$\begin{aligned} \Delta J_{1\pm} &= -\frac{D}{2} \rho_{1\pm}' \left[ G_x(x_1^-; x_1) + G_x(x_1^+; x_1) \right] \\ &= -\frac{1}{2} \delta L \frac{\sinh(2\kappa x_1/L)}{\sinh(\kappa)} \rho_{1\pm}' \ . \end{aligned} \tag{19}$$

Non-dimensionizing and Taylor expanding around $\kappa = 0$ we obtain,

$$\frac{\Delta J_{1\pm}}{c\delta L} = -\frac{\left(1 \pm \sqrt{1 - 4\sigma}\right)}{2} \frac{x_1}{L} + \mathcal{O}(\kappa^2) \ . \tag{20}$$

Hence, in the limit $\kappa \ll 1$ we find a similar linear dependence of the flux-differential on the sink position $x_1$ as for the 'non-inverted' case discussed earlier.
In the limit $\sigma \to 0$, the non-trivial solution of $\rho_1'$ is

$$\rho_1' = \frac{c}{G(x_1; x_1)}. \tag{21}$$

The derivative of the mass with respect to the spike position $x_1$ is,

$$\begin{aligned} \frac{\partial M}{\partial x_1} &= \frac{\partial}{\partial x_1}(c - \rho_1') = \frac{c}{G(x_1; x_1)^2} \frac{\partial G(x_1; x_1)}{\partial x_1} \\ \implies \frac{\partial M}{\partial x_1} &= \frac{c}{G(x_1; x_1)^2} \frac{\sinh(2\kappa x_1/L)}{\sinh(\kappa)}. \end{aligned}$$

Then, in the limit $\sigma \to 0$ and $\kappa \ll 1$ the flux differential and mass derivative become,

$$\frac{\Delta J_1}{c\delta L} = -\frac{1}{2} \frac{\sinh(2\kappa x_1/L)}{\sinh(\kappa)}, \qquad \frac{D}{c\delta L} \frac{\partial M}{\partial x_1} = \frac{\sinh(2\kappa x_1/L)}{\sinh(\kappa)}.$$

Therefore, just like for point sinks, in this limit, the velocity of a single spike can be expressed equivalently as,

$$\frac{dx_1}{dt} = \nu \Delta J_1 = -\nu \frac{1}{2} D \frac{\partial M}{\partial x_1} \tag{22}$$

Note that $\sigma \to 0$ for spikes (inverted sinks) corresponds $\lambda \to \infty$ for point sinks.

**Dynamics of $n$ spikes**

Let us consider a solution to the Turing system consisting of $n$ arbitrarily positioned spikes. From Eq. (12) and Eq. (11) we have,

$$\rho_i' = \sigma \frac{c^2}{c - \sum_j \rho_j' G(x_i; x_j)}, \tag{23}$$

which form a set of $n$ algebraic equations dependent on the peak positions. As $\sigma \to 0$, the condition becomes

$$\rho'_i(c - \sum_j \rho'_j G(x_i; x_j)) = 0, \quad \forall i \ .$$

Since $\rho'_i = 0$ is a trivial solution (it corresponds to removing one spike from the system), we must have

$$c - \sum_j \rho'_j G(x_i; x_j) = 0, \quad \forall i \ .$$

Now taking $\kappa \ll 1$ we expand the above equation in powers of $\kappa$ and collect terms of lowest order. We have,

$$\rho'_{0j} = \frac{c}{n}, \tag{24}$$

where $\rho'_j = \rho'_{0j} + \rho'_{2j}\kappa^2 + O(\kappa^4)$ and $G(x_i; x_j) = G_0(x_i; x_j) + G_2(x_i; x_j)\kappa^2 + O(\kappa^4)$. Next collecting terms of order $\kappa^2$ we have,

$$c - \sum_j \rho'_{0j} G_2(x_i; x_j) - \sum_j \rho'_{2j} G_0(x_i; x_j) = 0, \tag{25}$$

as the dependence on $x_i$ only shows up in this order. We see that the above equation is similar to the case of point sinks in the limit $\lambda \gg 1$ and $\kappa \ll 1$ (see main text). Following similar arguments to that case (with $M = c - \sum_j \rho'_j$ and expansion of $M$ in powers of $\kappa$, $M = M_0 + M_2\kappa^2 + ...$) we find that the derivative of the mass with respect to $x_i$ is given by

$$\frac{D}{c\delta L}\frac{\partial M}{\partial x_i} = \frac{2}{n}\frac{\partial}{\partial x_i}\sum_{i,j} G_2(x_i; x_j) + O(\kappa^4), \tag{26}$$

$$= \frac{2}{nL}\left[x_i - \frac{L}{n}i + \frac{L}{2}(\frac{1}{n} + 1)\right] + O(\kappa^4). \tag{27}$$

The flux differential across a spike is given by

$$\Delta J_i = -\frac{D}{\delta L}\sum_j \rho'_j \left[G_x(x_i^+; x_j) + \frac{\kappa^2}{2L}\delta_{ij}\right].$$

Expanding the above expression lowest order in $\kappa$ and following the same steps as for point sinks, we find

$$\frac{\Delta J_i}{c\delta L} = -\frac{1}{L}\left[x_i - \frac{L}{n}i + \frac{L}{2}(\frac{1}{n} + 1)\right] + O(\kappa^2) \tag{28}$$

Hence, in the limit $\sigma \to 0$ and $\kappa \to 0$ the spike velocity can be written as,

$$\frac{dx_i}{dt} = \nu\Delta J_i = -\nu\frac{n}{2}D\frac{\partial M}{\partial x_i}. \tag{29}$$

We conclude that while the two definitions for the spike velocity (flux differential and mass potential) are different in general, they become identical in the limit $\sigma \to 0, \kappa \to 0$.

## PEAK MOVEMENT IN OTHER MODELS

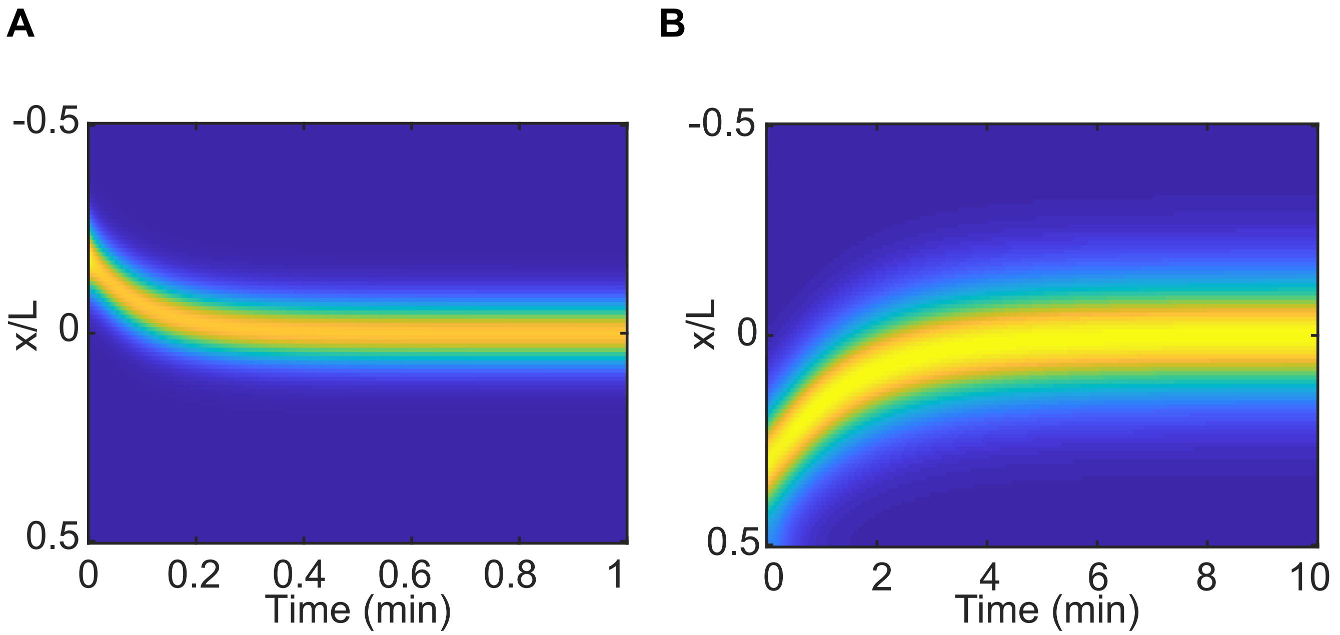


FIG. S6. **Peak movement in other reaction-diffusion system**.
($A$). Brusselator model. Kymograph of a single peak pattern moving exponentially to the mid-domain. Parameters: $a = 2, b = 0.001, \Gamma = 1500, d = 100$. ($B$). Kymograph of a single peak pattern in Schnakenberg model [2].

### MODELS WITH OTHER QUANTITIES FIXED AT STEADY STATE

In the Turing system considered here, the total combined mass of the system at steady state is fixed

$$\frac{1}{L}\int \bar{u}+\bar{v}\ dx = c\ . \tag{30}$$

Other systems such as the Brusselator [3] and the Schnakenberg model [2] have the integral of $\bar{v}$ being fixed. In our model, the individual integrals of $\bar{u}$ and $\bar{v}$ can vary and we have shown that the steady-sate reached by the system, after any coarsening, is determined by minimizing the integral of $\bar{u}$, the fast species.

Since our results indicate that minimization of the mass (integral) of the fast species is the determinant of pattern selection, it suggests that a Turing patterns may not be possible in a model that has the mass of $u$ fixed at steady state. Let us consider a general class of Turing systems of the following form

$$\partial_t u = D_u \partial_x^2 u - f(u,v) + a - g(u), \tag{31a}$$

$$\partial_t v = D_v \partial_x^2 v + f(u,v) + b. \tag{31b}$$

with $D_v < D_u$. We denote the stable fixed point of the homogeneous system by $(u_0, v_0)$. The functions $f(u,v)$ and $g(u)$ are arbitrary apart from the constraint that $g'(u_0) > 0$. The integral $\int g(\cdot)dx$ then acts a measure for $u$ and all steady state solutions $(\bar{u}, \bar{v})$ have the same mass of $u$ using this measure

$$\frac{1}{L}\int_{-L/2}^{L/2} g(\bar{u})dx = a + b.$$

The Jacobian at the homogeneous fixed point is given by,

$$J = \begin{bmatrix} -f_u - g_u & -f_v \\ f_u & f_v \end{bmatrix}\ , \tag{32}$$

where $f_u$, $f_v$ and $g_u$ are evaluated at the $(u_0, v_0)$. If the fixed point is stable we must have

$$TrJ = -f_u - g_u + f_v < 0$$
$$DetJ = -g_u f_v > 0\ .$$

The latter relation implies that $f_v < 0$. A necessary condition for a Turing instability (on an infinite domain) is that

$$-\frac{D_v}{D_u}(f_u + g_u) + f_v > 0. \tag{33}$$

However since $D_v < D_u$, this condition can never be satisfied. Hence, the general system Eq. (31) does not admit a Turing instability, consistent with our suggestion that mass minimisation of the fast species underlies pattern selection.


[1] J. D. Murray, *Mathematical Biology II - Spatial Models and Biomedical Applications*, edited by J. D. Murray, Interdisciplinary Applied Mathematics, Vol. 18 (Springer New York, New York, NY, 2003) p. 814.

[2] J. Schnakenberg, Simple chemical reaction systems with limit cycle behaviour, Journal of Theoretical Biology **81**, 389 (1979).

[3] I. Prigogine and R. Lefever, Symmetry breaking instabilities in dissipative systems. II, The Journal of Chemical Physics **48**, 1695 (1968).
